# Supplementary material for: Increased peak detection accuracy in over-dispersed ChIP-seq data with supervised segmentation models
Source: arXiv:2012.06848 source file (2020-12-15)
Supplement: Supplementary file 1 [file supplement.pdf]

# Increased peak detection accuracy in over-dispersed ChIP-seq data with supervised segmentation models
*(Supplementary Materials)*

Arnaud Liehrmann, arnaud.lieh@gmail.com *†
Guillem Rigaill, guillem.rigaill@inrae.fr *†
Toby Dylan Hocking, toby.hocking@nau.edu ‡

| datasets | type of ChIP-Seq experiment | number of folds |
|---|---|---|
| H3K36me3_AM_immune | H3K36me3 (broad peaks) | 10 |
| H3K36me3_TDH_immune | H3K36me3 (broad peaks) | 4 |
| H3K36me3_TDH_other | H3K36me3 (broad peaks) | 4 |
| H3K4me3_PGP_immune | H3K4me3 (sharp peaks) | 10 |
| H3K4me3_TDH_immune | H3K4me3 (sharp peaks) | 10 |
| H3K4me3_TDH_other | H3K4me3 (sharp peaks) | 10 |
| H3K4me3_XJ_immune | H3K4me3 (sharp peaks) | 10 |

Table 1: Summary of the number of folds in the cross-validation procedure by dataset.

*Université Paris-Saclay, CNRS, INRAE, Univ Evry, Institute of Plant Sciences Paris-Saclay (IPS2), Orsay, 91405 France.

†Université Paris-Saclay, CNRS, Univ Evry, Laboratoire de Mathématiques et Modélisation d'Evry, Evry, France.

‡Northern Arizona University, School of Informatics, Computing, and Cyber Systems 1295 S. Knoles Dr., Building 90, Room 210, Flagstaff, AZ, 86011, USA.

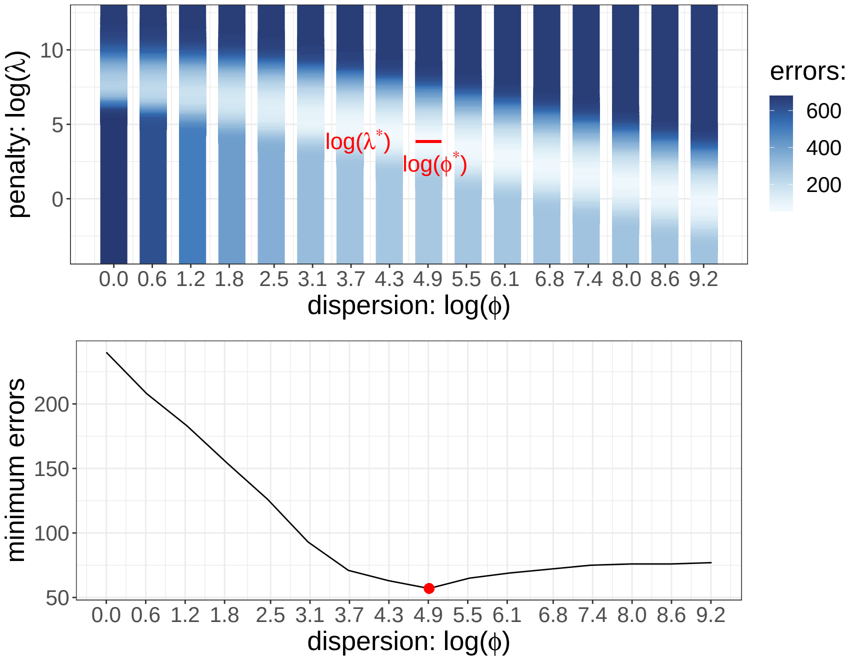


Figure 1: (**Top**) Visualization of $\sum_{m\in \text{ training set}} E_m(\phi \in \Phi, \lambda)$. The global minimum error (57), shown in red (■), is reached for $\lambda^* = 46.86$ and $\phi^* = 135.94$. (**Bottom**) For each $\phi_i$, i.e 16 values evenly placed on the log scale between 1 and 10000, the minimum error of $E_m(\phi_i, \lambda)$ has been plotted. We can see the errors growing constantly at the left en right side of $\phi^*$ which suggests that this range of $\phi$ is appropriate for learning a suitable dispersion parameter value.

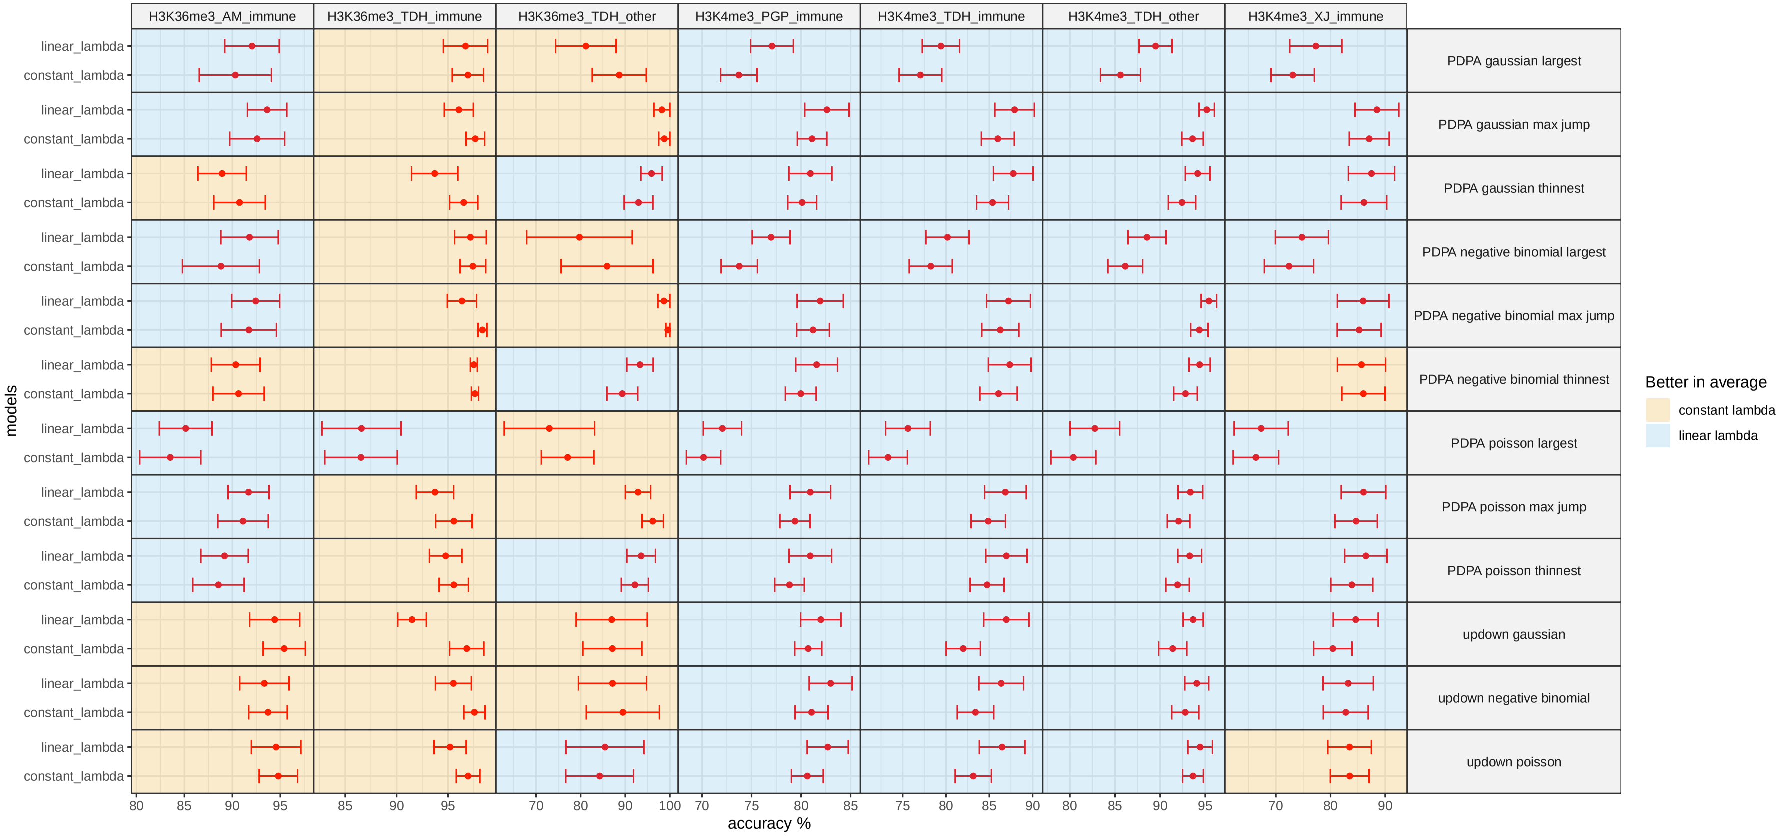


Figure 2: The *linear* $\lambda$ learning method improves the accuracy of the segmentation models upon the *constant* $\lambda$ learning method on H3K4me3 datasets. The mean accuracy and its 95% CI computed on the test folds is shown in red (■). In 46 of the 48 comparisons on the H3K4me3 datasets, the *linear* $\lambda$ learning method was better in average than the *constant* $\lambda$ learning method. After pooling the folds by type of experiment, we performed a paired t-test on each comparison. After correcting the p-values with the Benjamini & Hochberg method, 6 (/12) differences in mean accuracy were still significant (adjusted p-value $< 0.05$). The concerned models are: PDPA gaussian max jump; PDPA gaussian largest; PDPA negative binomial largest; PDPA poisson thinnest; updown gaussian; updown negative binomial. In H3K36me3 datasets, there is no clear trend on which learning method is the best. 24 of the 36 comparisons are in favour of the *constant* $\lambda$ learning method. After pooling the folds by type of experiment and performed a paired t-test following by a correction of the p-values, none of the 12 differences in mean were significant.
